# Supplementary material for: On the Precise Asymptotics of Universal Inference
Source: arXiv:2503.14717 source file (2025-03-18)
Supplement: Supplementary file 1 [file convex.tex]

\newpage
\section{Revising the proof of Theorem~\ref{thm:concentration-width-unbounded}}
We replace \ref{as:margin} as follows:

We assume that $\theta \mapsto Pm_{\theta}$ is convex. Furthermore, there exists constants $\delta > 0$ and $C$ such that $P(m_{\theta}-m_{\theta_0})\ge C\|\theta-\theta_0\|^{1+\beta}$ for all $\|\theta - \theta_0\| \le \delta$.

For any $\theta = \theta_0 + \ell u$ with $u \in \Theta$ such that $\|u\|=1$ and $\ell > \delta$, we define $\bar\theta = \theta_0 + \ell u$. Since $\bar\theta = (1-\delta/\ell)\theta_0 + \delta/\ell \theta$, it follows by the convexity
\begin{align*}
     (1-\delta/\ell) Pm_{\theta_0} - \delta/\ell Pm_{\theta} \ge Pm_{\bar \theta} \Longleftrightarrow  Pm_{\theta}-Pm_{\theta_0}  \ge (\ell/\delta)(Pm_{\bar \theta} -Pm_{\theta_0}) \ge \|\theta-\theta_0\|\delta^{\beta}.
\end{align*}
Hence we have a lower bound for all $\theta \in \Theta$ such that 
\begin{align*}
    P(m_{\theta}-m_{\theta_0})\ge C\left(\|\theta-\theta_0\|^{1+\beta} \wedge \|\theta-\theta_0\|\delta^{\beta}\right).
\end{align*}
\kt{
Any $\vartheta \in \widehat{\mathrm{CI}}$ satisfies 
\begin{align*}
    &\mathbb{P}_n(m_{\vartheta} - m_{\widehat{\theta}}) - q_{1-\alpha}n^{-1/2}\widehat\sigma_{\vartheta, \widehat{\theta}} \le 0 \\
    &\qquad \Longleftrightarrow P(m_{\vartheta} - m_{\theta_0}) + (\mathbb{P}_n-P)(m_{\vartheta} - m_{\theta_0}) - q_{1-\alpha}n^{-1/2}\widehat\sigma_{\vartheta, \theta_0} \le \mathbb{P}_n(m_{\widehat{\theta}} - m_{\theta_0}) + q_{1-\alpha}n^{-1/2}\widehat\sigma_{\widehat{\theta},\theta_0}
\end{align*}
We can further lower bound 
\begin{align*}
    &P(m_{\vartheta} - m_{\theta_0}) + (\mathbb{P}_n-P)(m_{\vartheta} - m_{\theta_0}) - q_{1-\alpha}n^{-1/2}\widehat\sigma_{\vartheta, \theta_0} \\
    &\qquad \ge  C\delta^\beta \|\vartheta-\theta_0\| + (\mathbb{P}_n-P)\frac{m_{\vartheta} - m_{\theta_0}}{\sigma_{\vartheta, \theta_0}}\sigma_{\vartheta, \theta_0} - \frac{n^{-1/2}\widehat\sigma_{\vartheta, \theta_0}}{\sigma_{\vartheta, \theta_0}}\sigma_{\vartheta, \theta_0}\\
    &\qquad \ge  C\delta^\beta \|\vartheta-\theta_0\| -C\left|(\mathbb{P}_n-P)\frac{m_{\vartheta} - m_{\theta_0}}{\sigma_{\vartheta, \theta_0}}\right|\|\vartheta-\theta_0\|^\alpha - C\left|\frac{n^{-1/2}\widehat\sigma_{\vartheta, \theta_0}}{\sigma_{\vartheta, \theta_0}}\right|\|\vartheta-\theta_0\|^\alpha\\
    &\qquad \ge  C\delta^\beta \|\vartheta-\theta_0\| -Cn^{-1/2}\sup_{\vartheta \in \Theta}\left|\mathbb{G}_n\frac{m_{\vartheta} - m_{\theta_0}}{\sigma_{\vartheta, \theta_0}}\right|\|\vartheta-\theta_0\|^\alpha \\
    &\qquad\qquad- Cn^{-1/2}\sup_{\vartheta \in \Theta}\left|\frac{\widehat\sigma_{\vartheta, \theta_0}}{\sigma_{\vartheta, \theta_0}}-1\right|\|\vartheta-\theta_0\|^\alpha -Cn^{-1/2} \|\vartheta-\theta_0\|^\alpha
\end{align*}
}

Next, we let 
\begin{align*}
    f(\theta) = P(m_{\theta} - m(\widehat{\theta})) \quad \text{and}\quad g(\theta) = P(m_{\theta} - m(\widehat{\theta})) - q_{1-\alpha}n^{-1/2}\sigma_{\theta, \theta_0}
\end{align*}
Any $\vartheta \in \widehat{\mathrm{CI}}$ satisfies 
\begin{align*}
    &\mathbb{P}_n(m_{\vartheta} - m(\widehat{\theta})) - q_{1-\alpha}n^{-1/2}\widehat\sigma_{\vartheta, \widehat{\theta}} \le 0 \\
    &\qquad \Longleftrightarrow g(\vartheta) \le (P_0-\mathbb{P}_n)(m_{\vartheta} - m(\widehat{\theta})) + q_{1-\alpha}n^{-1/2}\left(\widehat\sigma_{\vartheta, \widehat{\theta}}-\sigma_{\vartheta, \theta_0}\right)\\
    &\qquad \Longleftrightarrow g(\vartheta) -g(\theta_0)\le (P_0-\mathbb{P}_n)(m_{\vartheta} - m_{\widehat{\theta}}) + q_{1-\alpha}n^{-1/2}\left(\widehat\sigma_{\vartheta, \widehat{\theta}}-\sigma_{\vartheta, \theta_0}\right)-g(\theta_0)
\end{align*}
The last inequality further implies that 
\begin{align*}
    &g(\vartheta) -g(\theta_0)\\
    &\qquad \le |(P_0-\mathbb{P}_n)(m_{\vartheta} - m_{\widehat{\theta}})| + q_{1-\alpha}n^{-1/2}\left|\widehat\sigma_{\vartheta, \theta_0}-\sigma_{\vartheta, \theta_0}\right| + q_{1-\alpha}n^{-1/2} \widehat\sigma_{\theta_0, \widehat{\theta}}+ |P(m_{\theta_0} - m_{\widehat{\theta}})|.
\end{align*}
Combining the lower bound for $f$, we have 
\begin{align*}
    C\left(\|\vartheta-\theta_0\|^{1+\beta} \wedge \|\vartheta-\theta_0\|\delta^{\beta}\right) &\le f(\vartheta)-f(\theta_0) \\
     &= \{f(\vartheta)-g(\vartheta)\}-\{f(\theta_0)-g(\theta_0)\} + g(\vartheta) - g(\theta_0)\\
     &= q_{1-\alpha}n^{-1/2}\sigma_{\vartheta, \theta_0}+ |(P_0-\mathbb{P}_n)(m_{\vartheta} - m_{\widehat{\theta}})| + q_{1-\alpha}n^{-1/2}\left|\widehat\sigma_{\vartheta, \theta_0}-\sigma_{\vartheta, \theta_0}\right| \\
     &\qquad + q_{1-\alpha}n^{-1/2} \widehat\sigma_{\theta_0, \widehat{\theta}}+ |P(m_{\theta_0} - m_{\widehat{\theta}})|\\
     &= q_{1-\alpha}n^{-1/2}\left(\sigma_{\vartheta, \theta_0}+ |q_{1-\alpha}^{-1}\mathbb{G}_n(m_{\vartheta} - m_{\widehat{\theta}})| +\left|\widehat\sigma_{\vartheta, \theta_0}-\sigma_{\vartheta, \theta_0}\right|\right) \\
     &\qquad + q_{1-\alpha}n^{-1/2} \widehat\sigma_{\theta_0, \widehat{\theta}}+ |P(m_{\theta_0} - m_{\widehat{\theta}})|\\
     &= q_{1-\alpha}n^{-1/2}\left(\sigma_{\vartheta, \theta_0}+ |q_{1-\alpha}^{-1}\mathbb{G}_n(m_{\vartheta} - m_{\widehat{\theta}})| +\left|\widehat\sigma_{\vartheta, \theta_0}-\sigma_{\vartheta, \theta_0}\right|\right) \\
     &\qquad + \mathrm{R}_n(\widehat{\theta}, \theta_0)
\end{align*}

Recall 
\begin{align*}
    \sigma_{\vartheta, \theta_0} = \sqrt{\E(m_{\vartheta}-m_{\theta_0})^2 - (\E[m_{\vartheta}-m_{\theta_0}])^2} \le \sqrt{\E(m_{\vartheta}-m_{\theta_0})^2} 
\end{align*}
for the case of quantile estimation, we have 
\begin{align*}
   \sqrt{\E(m_{\vartheta}-m_{\theta_0})^2}  \le \sqrt{6}|\vartheta-\theta|
\end{align*}
Using the Markov inequality, we can claim the second term in the parenthesis is bounded in high probability by  $(2+\alpha)|\vartheta-\theta|$, which comes from
\begin{align*}
    	\E_P \left[\sup_{\|\theta-\theta(P)\| < \delta}|\mathbb{G}_n (m_\theta - m_{\theta(P)})| \right]\le(2+\alpha)\delta.
    \end{align*}

Finally, 
\begin{align*}
    |\widehat\sigma_{\vartheta, \theta_0}-\sigma_{\vartheta, \theta_0}| &= \sqrt{\widehat\sigma^2_{\vartheta, \theta_0}-\sigma^2_{\vartheta, \theta_0}+ \sigma^2_{\vartheta, \theta_0}}-\sigma_{\vartheta, \theta_0} \\
    &\le \sqrt{|\widehat\sigma^2_{\vartheta, \theta_0}-\sigma^2_{\vartheta, \theta_0}|}
\end{align*}
We also have 
\begin{align*}
    \widehat\sigma^2_{\vartheta, \theta_0} \le \mathbb{P}_n(m_{\vartheta}-m_{{\theta}_0})^2 \quad \textrm{and} \quad \sigma^2_{\vartheta, \theta_0} = P(m_{\vartheta}-m_{{\theta}_0})^2-\{P(m_{\vartheta}-m_{{\theta}_0})\}^2
\end{align*}
Hence, we have 
\begin{align*}
     |\widehat\sigma_{\vartheta, \theta_0}-\sigma_{\vartheta, \theta_0}| &\le \sqrt{(\mathbb{P}_n-P)(m_{\vartheta}-m_{{\theta}_0})^2} + |P(m_{\vartheta}-m_{{\theta}_0})|\\
     &\le \sqrt{(\mathbb{P}_n-P)(m_{\vartheta}-m_{{\theta}_0})^2} + \sqrt{P(m_{\vartheta}-m_{{\theta}_0})^2}
\end{align*}
The last term is already adressed. We have also shown that the first term is bounded in high probablity by $\sqrt{C}(2+\alpha)|\vartheta-\theta_0|$, which comes again from the Markov inequality and controlling on the squared empirical process.

In summary, we have 
\begin{align*}
     C|\theta-\theta_0|\delta^{\beta} \le q_{1-\alpha}n^{-1/2}\left(\sqrt{C_\varepsilon}(2+\alpha)|\theta-\theta_0|\right) + \mathrm{R}_n(\widehat{\theta}, \theta_0) 
\end{align*}
in probability $1-\varepsilon$ for all $\theta$ such that $|\theta-\theta_0|\le |\vartheta-\theta_0|$. \kt{Here, the logic is a bit questionable. This works when the empirical process terms all grow sublinearly. But when the upper bound grows faster, we should get an infinite confidence set.}

\kt{The assumption I am working with is essentially 
\begin{align*}
    &\E_P \left[\sup_{\delta \le \|\theta-\theta(P)\| < \Delta}|\mathbb{G}_n (m_\theta - m_{\theta(P)})| \right]  \vee \left\{n^{-1/2}\E_P \left[\sup_{\delta \le\|\theta-\theta(P)\| < \Delta}|\mathbb{G}_n (m_\theta - m_{\theta(P)})^2| \right]\right\}^{1/2} \\
    &\qquad \vee \left[\sup_{\delta \le\|\theta-\theta(P)\| < \Delta}\E_P(m_\theta - m_{\theta(P)})^2\right] \le C \Delta^\alpha \quad \text{for some $\alpha \in [0,1]$}
\end{align*}
I think the third one is redundant since the second term is bigger.
}
Then 
\begin{align*}
    &\left(C\delta^{\beta}- q_{1-\alpha}n^{-1/2}\sqrt{C_\varepsilon}(2+\alpha)\right)_+|\theta-\theta_0|\le \mathrm{R}_n(\widehat{\theta}, \theta_0) \\
    &\qquad \Longrightarrow  |\theta-\theta_0| \le \left(C\delta^{\beta}- q_{1-\alpha}n^{-1/2}\sqrt{C_\varepsilon}(2+\alpha)\right)_+^{-1}\mathrm{R}_n(\widehat{\theta}, \theta_0)
\end{align*}

For all $n$ such that 
\begin{align*}
    C\delta^{\beta}- q_{1-\alpha}n^{-1/2}\sqrt{C_\varepsilon}(2+\alpha) > 0 \Longrightarrow n> C^{-2}\delta^{-2\beta} q_{1-\alpha}^{2}C_\varepsilon(2+\alpha)^2
\end{align*}
For all $n$ greater than $C^{-2}\delta^{-2\beta} q_{1-\alpha}^{2}C_\varepsilon(2+\alpha)^2$, the radius is bounded up to a constant by $\delta^{-\beta}\mathrm{R}_n(\widehat{\theta}, \theta_0)$ in probability. 

\kt{as $\delta \to \infty$, this remainder term becomes zero and it holds with all $n \ge 1$.}

\kt{If we instead of defining $C\Delta^\alpha$ as $t \mapsto \omega(t)$ such that $\omega(t)/t^{\alpha}$ is non-increasing for all $t \ge \delta$ and $\alpha \in [0,1]$, then we can get a general result in the form of 
\begin{align*}
     &C|\theta-\theta_0|\delta^{\beta} \le q_{1-\alpha}n^{-1/2}\omega(|\theta-\theta_0|) + \mathrm{R}_n(\widehat{\theta}, \theta_0) \\
     &\qquad \Longrightarrow \left(C|\theta-\theta_0|\delta^{\beta} - q_{1-\alpha}n^{-1/2}\omega(|\theta-\theta_0|)  \right)_+\le \mathrm{R}_n(\widehat{\theta}, \theta_0)\\
     &\qquad \Longrightarrow \left(C|\theta-\theta_0|\delta^{\beta} - q_{1-\alpha}n^{-1/2}|\theta-\theta_0|^{\alpha}\delta^{-\alpha}\omega(\delta)  \right)_+\le \mathrm{R}_n(\widehat{\theta}, \theta_0)\\
     &\qquad \Longrightarrow |\theta-\theta_0|\left(C\delta^{\beta} - q_{1-\alpha}n^{-1/2}|\theta-\theta_0|^{\alpha-1}\delta^{-\alpha}\omega(\delta)  \right)_+\le \mathrm{R}_n(\widehat{\theta}, \theta_0)\\
     &\qquad \Longrightarrow |\theta-\theta_0|\left(C\delta^{\beta} - q_{1-\alpha}n^{-1/2}\delta^{-1}\omega(\delta)  \right)_+\le \mathrm{R}_n(\widehat{\theta}, \theta_0)
\end{align*}
Hence for all 
\begin{align*}
    n  > C^{-2}\delta^{-(2\beta)}q_{1-\alpha}^2(\omega(\delta)/\delta)^2
\end{align*}
the confidence width is bounded in probability by $\delta^{-\beta}\mathrm{R}_n(\widehat{\theta}, \theta_0)$. Putting together with the proof by peeling on $\|\theta-\theta_0\| \le \delta$, we get
\begin{align*}
    \min\left\{(r_n^2 \vee u_n\vee t_n \vee s_n)^{1/(1+\beta)}, \delta \right\} + \delta^{-\beta}\mathrm{R}_n(\widehat{\theta}, \theta_0)
\end{align*}
}
\newpage
\section{Another attempt}
Let $\{T_n\}$ be a non-random divergent sequence. We show that 
\begin{align*}
    \widehat{\mathrm{CI}}_{n, \alpha} \cap B(\theta_0; T_n) \subseteq B(\theta_0; \gamma_{n,\varepsilon})
\end{align*}
for some $\gamma_{n,\varepsilon} \longrightarrow 0$ with probability greater than $1-\varepsilon$. By the convexity, we obtain a lower bound for all $\theta \in \Theta$ such that 
\begin{align*}
    P(m_{\theta}-m_{\theta_0})\ge C\left(\|\theta-\theta_0\|^{1+\beta} \wedge \|\theta-\theta_0\|\delta^{\beta}\right).
\end{align*}
We now assume that 
\begin{align*}
    |m_{\theta}(Z) - m_{\theta_0}(Z)| \le g(Z)\|\theta-\theta_0\|^\nu
\end{align*}
for some random variable $g$ and $\nu \in (0,1]$. We assume that $g$ is $P_q$-integrable, i.e., $\int |g|^q\, dP < \infty$ for some $q \ge 2$. 
Any $\theta \in \widehat{\mathrm{CI}}$ satisfies 
\begin{align*}
    &\mathbb{P}_n(m_{\theta} - m_{\widehat{\theta}}) - q_{1-\alpha}n^{-1/2}\widehat\sigma_{\theta, \widehat{\theta}} \le 0 \\
    &\qquad \Longleftrightarrow P(m_{\theta} - m_{\theta_0}) + (\mathbb{P}_n-P)(m_{\theta} - m_{\theta_0}) \le \mathbb{P}_n(m_{\widehat{\theta}} - m_{\theta_0}) + q_{1-\alpha}n^{-1/2}\widehat\sigma_{\widehat{\theta},\theta}\\
    &\qquad \Longrightarrow P(m_{\theta} - m_{\theta_0}) + (\mathbb{P}_n-P)(m_{\theta} - m_{\theta_0}) \\
    &\qquad\qquad \le \mathbb{P}_n(m_{\widehat{\theta}} - m_{\theta_0}) + q_{1-\alpha}n^{-1/2}\|g\|_{L_2(\mathbb{P}_n)}\left(\|\theta-\theta_0\|+ \|\widehat{\theta}-\theta_0\|\right)^\nu\\
    &\qquad \Longrightarrow P(m_{\theta} - m_{\theta_0}) + (\mathbb{P}_n-P)(m_{\theta} - m_{\theta_0}) \\
    &\qquad\qquad \le \mathbb{P}_n(m_{\widehat{\theta}} - m_{\theta_0}) + q_{1-\alpha}n^{-1/2}\|g\|_{L_2(\mathbb{P}_n)}\left(\|\theta-\theta_0\|+ \|\widehat{\theta}-\theta_0\|\right)^\nu 
\end{align*}
We now split into cases. First, when $P(m_{\theta} - m_{\theta_0}) \le r_n^2$ (to be defined), we have 
\begin{align*}
    C\left(\|\theta-\theta_0\|^{1+\beta} \wedge \|\theta-\theta_0\|\delta^{\beta}\right) \le r_n^2 \Longrightarrow \|\theta-\theta_0\| \lesssim_{C}  r_n^2/\delta^{\beta}+  r_n^{2/(1+\beta)}
\end{align*}
Next, when $P(m_{\theta} - m_{\theta_0}) > r_n^2$, we have 
\begin{align*}
    & P(m_{\theta} - m_{\theta_0}) + (\mathbb{P}_n-P)(m_{\theta} - m_{\theta_0}) \\
    &\qquad\qquad \le \mathbb{P}_n(m_{\widehat{\theta}} - m_{\theta_0}) + q_{1-\alpha}n^{-1/2}\|g\|_{L_2(\mathbb{P}_n)}\left(\|\theta-\theta_0\|+ \|\widehat{\theta}-\theta_0\|\right)^\nu\\
    &\qquad \Longleftrightarrow P(m_{\theta} - m_{\theta_0}) \left(1 + \frac{(\mathbb{P}_n-P)(m_{\theta} - m_{\theta_0})}{P(m_{\theta} - m_{\theta_0})}\right) \\
    &\qquad\qquad \le \mathbb{P}_n(m_{\widehat{\theta}} - m_{\theta_0}) + q_{1-\alpha}n^{-1/2}\|g\|_{L_2(\mathbb{P}_n)}\left(\|\theta-\theta_0\|+ \|\widehat{\theta}-\theta_0\|\right)^\nu\\
    &\qquad \Longrightarrow C\left(\|\theta-\theta_0\|^{1+\beta} \wedge \|\theta-\theta_0\|\delta^{\beta}\right) \left(1 - \sup_{\theta \in \Theta; P(m_{\theta} - m_{\theta_0}) > r_n}\left|\frac{(\mathbb{P}_n-P)(m_{\theta} - m_{\theta_0})}{P(m_{\theta} - m_{\theta_0})}\right|\right)_+ \\
    &\qquad\qquad \le \mathbb{P}_n(m_{\widehat{\theta}} - m_{\theta_0}) + q_{1-\alpha}n^{-1/2}\|g\|_{L_2(\mathbb{P}_n)}\left(\|\theta-\theta_0\|+ \|\widehat{\theta}-\theta_0\|\right)^\nu
\end{align*}
For a moment, we assume that 
\[\sup_{\theta \in \Theta; P(m_{\theta} - m_{\theta_0}) > r_n^2}\left|\frac{(\mathbb{P}_n-P)(m_{\theta} - m_{\theta_0})}{P(m_{\theta} - m_{\theta_0})}\right| \le C_\varepsilon < 1\]
with probability greater than $1-\varepsilon$. Then we have 
\begin{align*}
    &C_\varepsilon\left(\|\theta-\theta_0\|^{1+\beta} \wedge \|\theta-\theta_0\|\delta^{\beta}\right) \le \mathbb{P}_n(m_{\widehat{\theta}} - m_{\theta_0}) \\
    &\qquad\qquad+ q_{1-\alpha}n^{-1/2}\|g\|_{L_2(P)}\left(\|\theta-\theta_0\|+ \|\widehat{\theta}-\theta_0\|\right)^\nu.
\end{align*}
When $\|\theta-\theta_0\| > \delta$, we have 
\begin{align*}
    C_\varepsilon\|\theta-\theta_0\|\delta^{\beta} \le \mathbb{P}_n(m_{\widehat{\theta}} - m_{\theta_0}) + q_{1-\alpha}n^{-1/2}\|g\|_{L_2(P)}\left(\|\theta-\theta_0\|+ \|\widehat{\theta}-\theta_0\|\right)^\nu.
\end{align*}
Requiring that $\nu \le 1$, we have 
\begin{align*}
    &\|\theta-\theta_0\|\left(C_\varepsilon\delta^{\beta}- q_{1-\alpha}n^{-1/2}\|g\|_{L_2(P)}\delta^{\nu-1}\right)_+ \le \mathbb{P}_n(m_{\widehat{\theta}} - m_{\theta_0}) + q_{1-\alpha}n^{-1/2}\|g\|_{L_2(P)}\|\widehat{\theta}-\theta_0\|^\nu\\
    &\qquad \Longrightarrow \|\theta-\theta_0\| \le \frac{\mathbb{P}_n(m_{\widehat{\theta}} - m_{\theta_0}) + q_{1-\alpha}n^{-1/2}\|g\|_{L_2(P)}\|\widehat{\theta}-\theta_0\|^\nu}{\left(C_\varepsilon\delta^{\beta}- q_{1-\alpha}n^{-1/2}\|g\|_{L_2(P)}\delta^{\nu-1}\right)_+} \wedge T_n
\end{align*}

When $\|\theta-\theta_0\| < \delta$, we can use the usual peeling. \kt{This means that \[|m_{\theta}(Z) - m_{\theta_0}(Z)| \le g(Z)\|\theta-\theta_0\|^\nu\] needs to hold only when $\|\theta - \theta_0\| > \delta$}

Finally, we need to consider the ratio limit process 
\begin{align*}
    \sup_{\theta \in \Theta; P(m_{\theta} - m_{\theta_0}) > r_n^2}\left|\frac{(\mathbb{P}_n-P)(m_{\theta} - m_{\theta_0})}{P(m_{\theta} - m_{\theta_0})}\right|
\end{align*}
Consider a function class:
\begin{align*}
    \mathcal{M}_j := \left\{m_{\theta}-m_{\theta_0}: 2^jr_n < \sqrt{P(m_{\theta} - m_{\theta_0})} \le 2^{j+1}r_n,\, \forall \theta \in \Theta \cap B(\theta_0; T_n)\right\}
\end{align*}
For any $j \ge 0$, we have 
\begin{align*}
    &\sup_{m \in \mathcal{M}_j}|(\mathbb{P}_n-P)m| \\
    &\qquad = \sup_{m \in \mathcal{M}_j}(\mathbb{P}_n-P)m\mathbf{1}\{|m(Z)| \le B_j\} + \sup_{m \in \mathcal{M}_j}|(\mathbb{P}_n-P)m\mathbf{1}\{|m(Z)| > B_n\}| 
\end{align*}
For the second term, 
\begin{align*}
    &\mathbb{P}\left(\bigcup_{j=0}^\infty \left\{\sup_{m \in \mathcal{M}_j}\left|\frac{(\mathbb{P}_n-P)m\mathbf{1}\{|m(Z)| > B_j\}}{Pm}\right| > \varepsilon/2\right\}\right) \\
    &\qquad \le \sum_{j=0}^\infty 
\mathbb{P}\left(\sup_{m \in \mathcal{M}_j}\left|(\mathbb{P}_n-P)m\mathbf{1}\{|m(Z)| > B_j\}\right| > 2^{2j}r_n^2\varepsilon/2 \right)\\
    &\qquad \le \sum_{j=0}^\infty 
\mathbb{P}\left(\sup_{m \in \mathcal{M}_j}(\mathbb{P}_n+P)\left|m\mathbf{1}\{|m(Z)| > B_j\}\right| > 2^{2j}r_n^2\varepsilon/2 \right)\\
    &\qquad \le \sum_{j=0}^\infty \frac{4\mathbb{E}\sup_{m \in \mathcal{M}_j}|m|^q}{2^{2j}r_n^2B_j^{q-1}\varepsilon}
% 4\mathbb{E}\left(\sup_{m \in \mathcal{M}_j}|m|^q\left|m\mathbf{1}\{|m(Z)| > B_j\}\right| > 2^{2j}r_n^2\varepsilon/2 \right)
\end{align*}
\kt{For the case with quantile, we have 
\begin{align*}
    \mathbb{E}\sup_{m \in \mathcal{M}_j}|m|^q\le T_n^q + \mathbb{E}|Z-\theta_0|^q
\end{align*}
This depends on $T_n$}

For the first term, by Bousquet's inequality, we have 
\begin{align*}
    &\sup_{m \in \mathcal{M}_j}(\mathbb{P}_n-P)m\mathbf{1}\{|m(Z)| \le B_j\} \\
    &\qquad\le \mathbb{E}\left[\sup_{m \in \mathcal{M}_j}(\mathbb{P}_n-P)m\mathbf{1}\{|m(Z)| \le B_j\}\right] \\
    &\qquad\qquad + \sqrt{\frac{2t}{n}\left(\nu^2 + 2B_j \mathbb{E}\left[\sup_{m \in \mathcal{M}_j}|(\mathbb{P}_n-P)m\mathbf{1}\{|m(Z)| \le B_j\}|\right] \right)} + \frac{B_j t}{3n}
\end{align*}
with probability greater than $1-\exp(-t)$. Here, $\nu^2 \ge \sup_{m \in \mathcal{M}_j} \mathrm{Var}[m]$. We take 
\begin{align*}
    \nu^2 = B_j \sup_{m \in \mathcal{M}_j} Pm
\end{align*}
and we have 
\begin{align*}
    &\sup_{m \in \mathcal{M}_j}(\mathbb{P}_n-P)m\mathbf{1}\{|m(Z)| \le B_j\} \\
    &\qquad\le \mathbb{E}\left[\sup_{m \in \mathcal{M}_j}|(\mathbb{P}_n-P)m\mathbf{1}\{|m(Z)| \le B_j\}|\right] \\
    &\qquad\qquad + \sqrt{\frac{2tB_j}{n}\left(\sup_{m \in \mathcal{M}_j} Pm + 2\mathbb{E}\left[\sup_{m \in \mathcal{M}_j}|(\mathbb{P}_n-P)m\mathbf{1}\{|m(Z)| \le B_j\}|\right] \right)} + \frac{B_j t}{3n}
\end{align*}
Thus for any $m \in \mathcal{M}_j$, we have 
\begin{align*}
    &\frac{(\mathbb{P}_n-P)m\mathbf{1}\{|m(Z)| \le B_j\}}{Pm}\\
    &\qquad\le \frac{\mathbb{E}\left[\sup_{m \in \mathcal{M}_j}|(\mathbb{P}_n-P)m\mathbf{1}\{|m(Z)| \le B_j\}|\right]}{P m} \\
    &\qquad\qquad+ \sqrt{\frac{2tB_j}{n 2^{2j}r_n^2}\left(4 + \frac{2\mathbb{E}\left[\sup_{m \in \mathcal{M}_j}|(\mathbb{P}_n-P)m\mathbf{1}\{|m(Z)| \le B_j\}|\right]}{Pm} \right)} + \frac{B_j t}{3n 2^{2j}r_n^2 }
\end{align*}
As long as $\sum_{j=1}^\infty \exp(-t_j)$ goes to zero, we can allow $t_j$ to vary over $j$. Take $t_j = 2^{2j}t$, we have 
\begin{align*}
    &\frac{(\mathbb{P}_n-P)m\mathbf{1}\{|m(Z)| \le B_j\}}{Pm}\\
    &\qquad\le \frac{\mathbb{E}\left[\sup_{m \in \mathcal{M}_j}|(\mathbb{P}_n-P)m\mathbf{1}\{|m(Z)| \le B_j\}|\right]}{P m} \\
    &\qquad\qquad+ \sqrt{\frac{2tB_j}{n r_n^2}\left(4 + \frac{2\mathbb{E}\left[\sup_{m \in \mathcal{M}_j}|(\mathbb{P}_n-P)m\mathbf{1}\{|m(Z)| \le B_j\}|\right]}{Pm} \right)} + \frac{B_j t}{3nr_n^2 }
\end{align*}
hold for all $j \ge 0$ with probability greater than 
\begin{align*}
    1-\sum_{j=0}^\infty \exp(-2^{2j}t) \ge 1-\frac{4}{3}\cdot\frac{2}{t}\exp(-t/2)
\end{align*}

\begin{align*}
    &\frac{(\mathbb{P}_n-P)m\mathbf{1}\{|m(Z)| \le B_j\}}{Pm}\\
    &\qquad\le \frac{\mathbb{E}\left[\sup_{m \in \mathcal{M}_j}|\mathbb{G}_nm\mathbf{1}\{|m(Z)| \le B_j\}|\right]}{n^{1/2}r_n^2} \\
    &\qquad\qquad+ \sqrt{\frac{2tB_j}{n r_n^2}\left(4 + \frac{2\mathbb{E}\left[\sup_{m \in \mathcal{M}_j}|\mathbb{G}_n m\mathbf{1}\{|m(Z)| \le B_j\}|\right]}{n^{1/2}r_n^2} \right)} + \frac{B_j t}{3nr_n^2 }
\end{align*}
\kt{It remains to control 
\begin{align*}
    \mathbb{E}\left[\sup_{m \in \mathcal{M}_j}|\mathbb{G}_n m\mathbf{1}\{|m(Z)| \le B_j\}|\right]
\end{align*}
where $\mathcal{M}_j = \left\{m_{\theta}-m_{\theta_0}: 2^{2j}r_n^2 < P(m_{\theta} - m_{\theta_0}) \le 2^{2j+2}r_n^2,\, \forall \theta \in \Theta \cap B(\theta_0; T_n)\right\}$. 
\begin{align*}
    &\mathbb{E}\left[\sup_{m \in \mathcal{M}_j}|(\mathbb{P}_n -P) m\mathbf{1}\{|m(Z)| \le B_j\}|\right] \\
    &\qquad \le 2\mathbb{E}\left[\mathbb{E}^\circ\left[\left[\sup_{m \in \mathcal{M}_j}\left|\frac{1}{n}\sum_{i=1}^n \epsilon_i m(Z_i)\mathbf{1}\{|m(Z_i)| \le B_j\}\right|\right] \bigg| Z_1, \ldots, Z_n \right]\right]
\end{align*}
By the Dudley’s integral entropy bound for Rademacher processes, we have 
\begin{align*}
    2Cn^{-1/2}\mathbb{E}\left[\int_0^{\Delta_n} \sqrt{\log N(\eta, \mathcal{M}_{j, B_j}, L_2(\mathbb{P}_n))}\, d\eta\right]
\end{align*}
where 
$\Delta_n = \sqrt{\sup_{m \in \mathcal{M}_j}\mathbb{P}_n m^2}$. 
\begin{align*}
    \mathbb{E}[\Delta_n] \le  \sqrt{\mathbb{E}\left[\sup_{m \in \mathcal{M}_j}\mathbb{P}_n m^2\right] }
    &=  \sqrt{B_j\mathbb{E}\left|\sup_{m \in \mathcal{M}_j}\mathbb{P}_n m - P_0 m \right| + B_jr_n^2 2^{j+1}}
\end{align*}
}
\kt{For quantile, we can show that 
}
