# Supplementary material for: On the Precise Asymptotics of Universal Inference
Source: arXiv:2503.14717 source file (2025-03-18)
Supplement: Supplementary file 3 [file supp-concentration.tex]

\section{Concentration inequalities}
